# Supplementary material for: Designing Adiabatic Quantum Optimization: A Case Study for the Traveling Salesman Problem
Source: arXiv:1702.06248 ancillary file (2017-02-21)
Supplement: Supplementary file 1 [file supplemental.pdf]

# Supplemental material for: Designing Adiabatic Quantum Optimization – A Case Study for the Traveling Salesman Problem

Bettina Heim,[1,2] Ethan W. Brown,[1,3] Dave Wecker,[2] and Matthias Troyer[1,2]

[1]*Theoretische Physik, ETH Zurich, 8093 Zurich, Switzerland*
[2]*Quantum Architectures and Computation Group, Microsoft Research, Redmond WA*
[3]*Mindi Technologies Ltd. 71-74 Shelton Street, Covent Garden, London, UK, WC2H 9JQ*

### a. *Traveling Salesman Problem and its Map to an Ising Spin Glass Problem*

Consider the traveling salesman problem (TSP) of finding the cheapest way of traveling $N$ cities. Our goal is to find a permutation $\tau \in S_N$, that minimizes the tour costs. Represented $\tau$ as $N \times N$ matrix $(\tau_{ij})$ with

$$\tau_{ij} = \begin{cases} 1 & \text{if city } i \text{ is the } j\text{-th city of the tour} \\ 0 & \text{otherwise} \end{cases}$$

the costs for the tour $\tau$ are given by

$$K = \sum_{t=1}^{N} d_{\tau^{-1}(t)\tau^{-1}(t+1)} = \sum_{i,j\neq i} \sum_t d_{ij} \tau_{it} \tau_{jt+1} \tag{1}$$

with $\tau^{-1}(N+1) := \tau^{-1}(1)$ and $d_{ij}$ the costs to travel from city $i$ to city $j$.

The solution to this problem can be formulate as the ground state of an Ising spin glass. All permutations $(\tau_{ij})$ can be represented as a ground state of the Hamiltonian

$$H_c(\eta) = \eta \left( \sum_i \left( (1 - \sum_j \frac{1}{2}(\sigma^z_{ij}+1))^2 + (1 - \sum_j \frac{1}{2}(\sigma^z_{ji}+1))^2 \right) \right) \tag{2}$$

Thus, adding this constraining Hamiltonian with a suitable prefactor $\eta$ to the cost Hamiltonian, solving the TSP is equivalent to finding the ground state of

$$H^{(perm)}_{TSP} = \frac{1}{4} \sum_{i,j,k} d_{ij} \sigma^z_{ik} \sigma^z_{jk+1} + \sum_s \left( \frac{\tilde{d}_{s(i,j)}}{2} + \eta(N-3) \right) \sigma^z_s + \frac{\eta}{4} \sum_{\langle s,s' \rangle} \sigma^z_s \sigma^z_{s'} + \text{const}$$

with $\tilde{d}_{s(i,j)} := \sum_{j\neq i} \frac{1}{2}(d_{ij} + d_{ji})$ for a spin $s(i,j)$ representing $\tau_{ij}$.

The last sum is over all neighboring spins, where we consider two spins to be neighbors, if they either represent the same city or the same time during the tour. Such a formulation requires $(N-1)^2$ spins, as we can fix city $N$ to be the last city in the tour, each of which has $2(N-2)$ neighbors. The prefactor $\eta$ has to be chosen large enough to ensure that the ground state indeed corresponds to a tour configuration.

An alternative way of mapping the TSP onto a spin glass problem is to use $N(N-1)$ spins to represent not the permutation, but the the travelled connections between cities. In the case of a symmetric TSP, ie. $d_{ij} = d_{ji} \; \forall \; i,j$, the number of required spins reduces to $\frac{1}{2}N(N-1)$. We expect each city to be connected to exactly two other cities. The constraining Hamiltonian implementing these requirements takes the form

$$H'_c(\eta) = \eta \sum_i \left(2 - \sum_{j\neq i} \frac{1}{2}(\sigma^z_{ij}+1)\right)^2 \text{ with } \sigma^z_{ij} = \sigma^z_{ji} \tag{3}$$

This constraint, however, does allow a tour consisting of several closed subtours instead of one tour connecting all cities. In certain cases, it may be desirable to know, when several smaller tours are cheaper to travel than one big tour. In that case the Ising Hamiltonian

$$H^{(graph)}_{TSP} = \sum_e \left( \frac{d_e}{2} + \eta(N-5) \right) \sigma^z_e + \frac{\eta}{4} \sum_{\langle e,e' \rangle} \sigma^z_e \sigma^z_{e'} + \text{const} \tag{4}$$

will serve our purpose. The last sum over neighboring spin pairs includes all pairs of spins representing connections with one common start or end point.

If we rather want to insist on exactly one closed loop, additional precautions will have to be taken.

The ground state of an Ising spin glass can be found by quantum annealing, where the system evolves according to a time dependent Hamiltonian

$$H(t) = (1 - \frac{t}{T}) H_0 + \frac{t}{T} H_{TSP} \text{ for } 0 \leq t \leq T \tag{5}$$

with $[H_0, H_{TSP}] \neq 0$. Provided the system is in its ground state at $t = 0$ the adiabatic theorem guarantees a transition into the ground state of $H_{TSP}$ for $T \to \infty$.

### b. *Transition Probabilities in Quantum Annealing*

Consider the transition probability for transitions between two states $\psi_0$ and $\psi_1$ that each represent a valid tour. Both states are then eigenstates of $H_{TSP}$. Assume the system is in a state $\psi_0$ at a time $t_0 \lesssim T$. The probability that the state at a time $t_0 + \Delta t \lesssim T$ is $\psi_1$, if we choose $H_0 = -C_0 \sum_e \sigma^x_e$, $\hbar = 1$, can be approximated by

$$P_{t_0}(\Delta t) = \prod_{j \in I_1} \sin^2\left( \frac{C_0}{T} |a(\omega_j)| \right) \prod_{k \in I_2} \cos^2\left( \frac{C_0}{T} |a(\omega_k)| \right) + \mathscr{O}(|I_1| + 2r) \text{ for } r \ll N \tag{6}$$

with

$$|a(\omega_k)|^2 = \left( \frac{4}{\omega_k^4} + \frac{4t_0(t_0+\Delta t)}{\omega_k^2} \right) \sin^2\left(\frac{\omega_k}{2}\Delta t\right) + \frac{\Delta t^2}{\omega_k^2} - \frac{4\Delta t}{\omega_k^3} \sin\left(\frac{\omega_k}{2}\Delta t\right) \cos\left(\frac{\omega_k}{2}\Delta t\right) \tag{7}$$

The set $I_1$ contains all spins whose state differs between the two valid tours, $I_2$ all remaining spins. The terms $\omega_k$ are the frequencies belonging to the transition given by flipping spin $k$. While they depend on the state of the surrounding spins, we can neglect this dependency for term up to order $\mathcal{O}(|I_1|+2r)$ for $r \ll N$. We thus made the approximation that the frequencies $\omega_k$ are independent on the transition path from $\psi_0$ to $\psi_1$ in eq. 7.

In the limit $T \to \infty$, const $= \frac{\Delta t}{T} \ll 1$, the lowest order contribution to the transition amplitude simplifies to

$$A^{(s)}(\Delta t) = \Big(\frac{C_0 \Delta t}{T}\Big)^s \sum_{\substack{\text{shortest} \\ \text{paths } \gamma}} \prod_{m=1}^{s} \frac{1}{E_0 - E^{\perp}_{\gamma_m}} \tag{8}$$

where $s$ is the minimal path length to transition between the two states. The energies $E^{\perp}_{\gamma_m}$ are the eigenvalues of the intermediate states along the transition path, and thus path dependent.

| | **permutation mapping** | **graph mapping** |
|---|---|---|
| minimal number of required spin flips | $4\lfloor \frac{r+1}{2} \rfloor$ | $4r$ |
| maximal number of required spin flips | $2\big(N - \lceil \frac{N-(r-1)}{r+1} \rceil\big)$ | $4r$ |

Table I. Required number of spin flips to resolve $r$ crossings in the symmetric TSP compared for both mappings

Independent on the exact dynamics induced by $H_0$, the transition probability declines exponentially with the required number of moves for a transition between two given states. While this number is approximately the same for both mappings in the asymmetric case, the second map has a clear advantage in the symmetric case. Table I gives an overview for the number of single spin flips required to resolve $r$ crossings in both mappings.
